# Supplementary material for: DrivingSphere: Building a High-fidelity 4D World for Closed-loop Simulation
Source: arXiv:2411.11252 source file (2024-11-18)
Supplement: Supplementary file 1 [file X_suppl.tex]

\clearpage
\setcounter{page}{1}
\maketitlesupplementary

\section{Rationale}
\label{sec:rationale}
Having the supplementary compiled together with the main paper means that:
\begin{itemize}
\item The supplementary can back-reference sections of the main paper, for example, we can refer to \cref{sec:intro};
\item The main paper can forward reference sub-sections within the supplementary explicitly (e.g. referring to a particular experiment); 
\item When submitted to arXiv, the supplementary will already included at the end of the paper.
\end{itemize}
To split the supplementary pages from the main paper, you can use \href{https://support.apple.com/en-ca/guide/preview/prvw11793/mac#:~:text=Delete%20a%20page%20from%20a,or%20choose%20Edit%20%3E%20Delete).}{Preview (on macOS)}, \href{https://www.adobe.com/acrobat/how-to/delete-pages-from-pdf.html#:~:text=Choose%20%E2%80%9CTools%E2%80%9D%20%3E%20%E2%80%9COrganize,or%20pages%20from%20the%20file.}{Adobe Acrobat} (on all OSs), as well as \href{https://superuser.com/questions/517986/is-it-possible-to-delete-some-pages-of-a-pdf-document}{command line tools}.

\begin{table}[ht]
    \centering
    \begin{tabular}{c|c|c}
    \hline
    {Methods}     &$\text{IoU}_{\small(\uparrow)}$ &{$\text{mIoU}_{\small(\uparrow)}$}  \\
    \hline
    % LiDARGAN  & - & $30.6$ & -\\
    OccWorld & 62.29& 66.38 \\
    OccSora & 27.4 &37 \\
    UrbanDiff & 98.8 &80 \\
    \hline
    \ourmodel & 99 & 86.81 \\
    \hline
    \end{tabular}%
    \caption{\textbf{Quantitative results of VAE in Occupancy Generation.}}
    \label{tab:sota_s}
\end{table}

\begin{figure}
    \centering
    \includegraphics[width=0.5\linewidth]{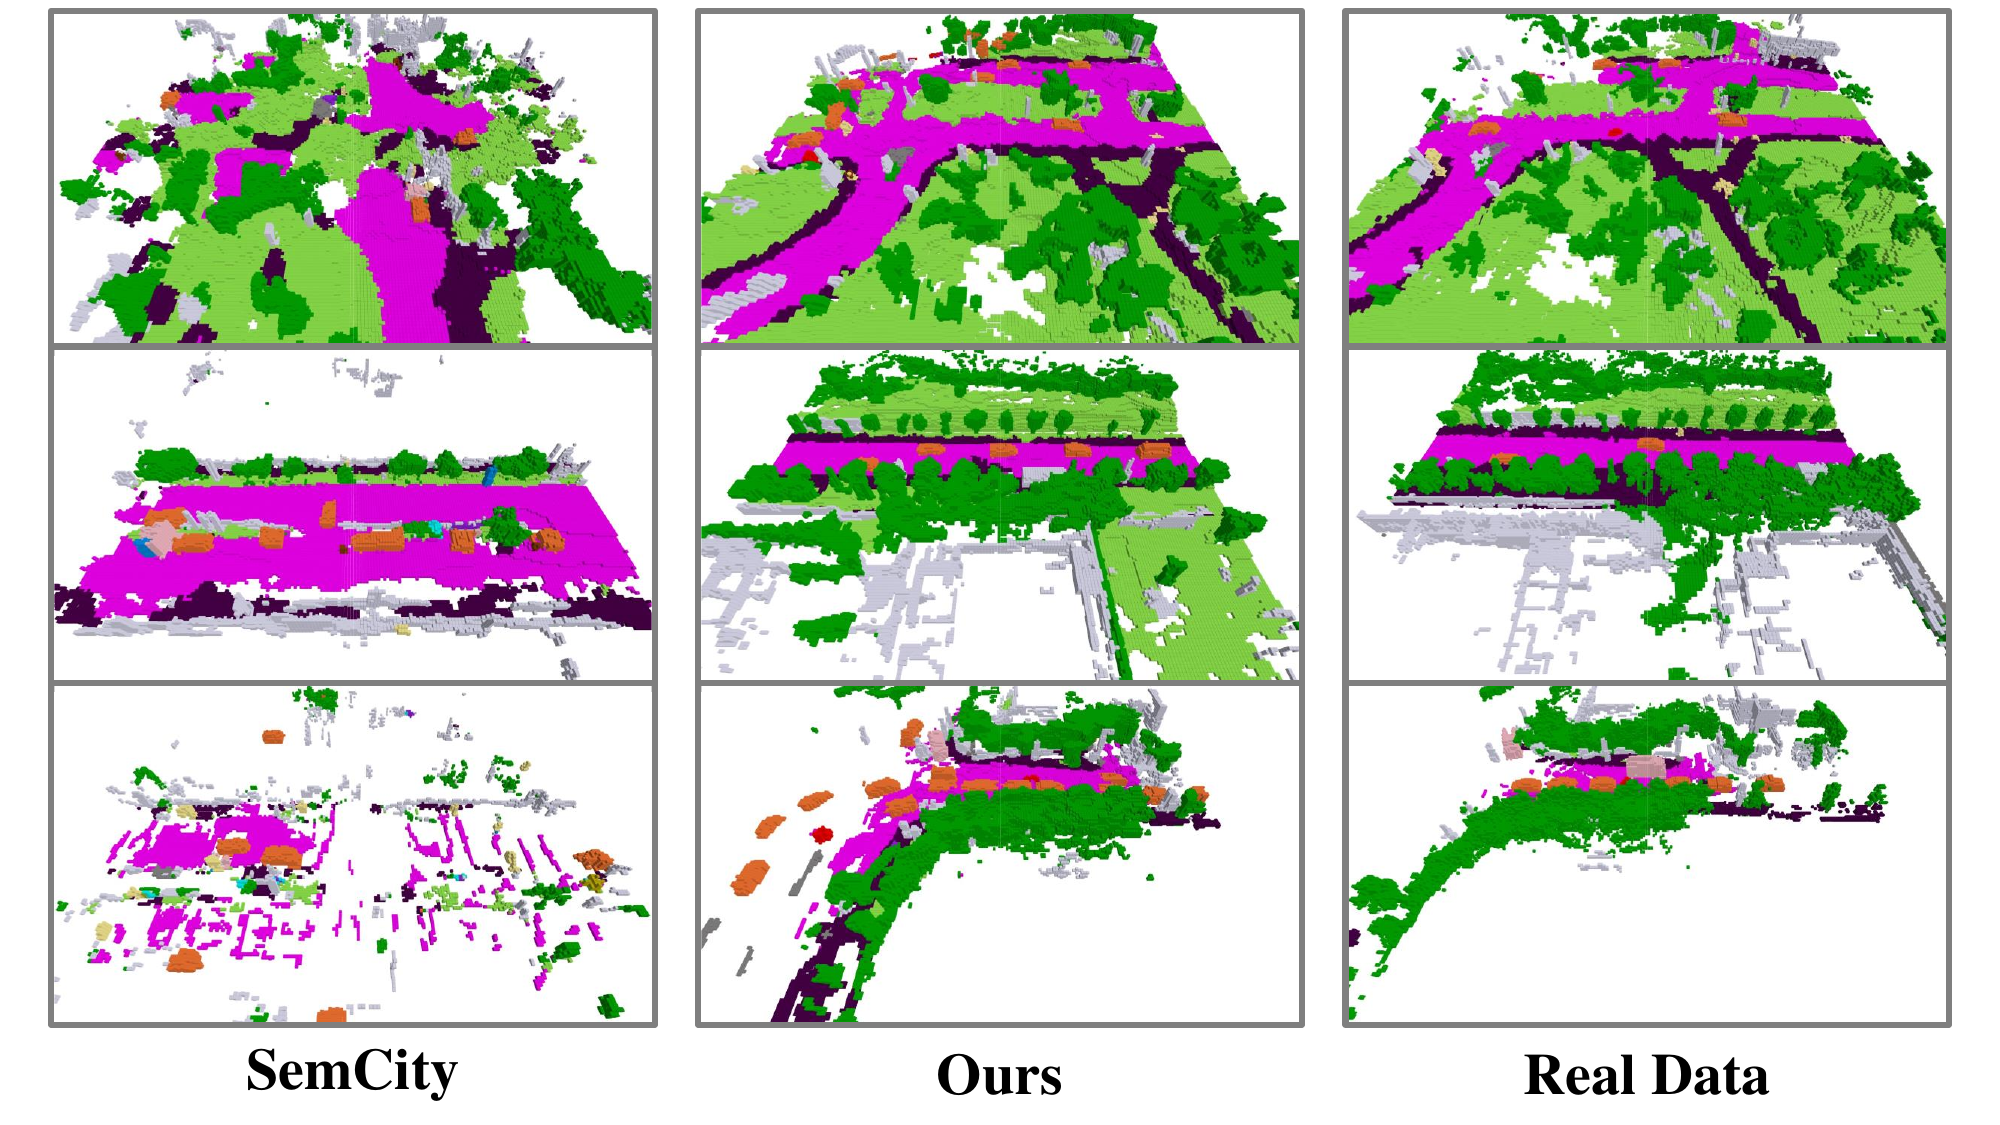}
    \caption{Caption}
    \label{fig:enter-label}
\end{figure}

\section{Training details}
occdreamer
videodreamer
closed loop
evaulation details

\section{network details}

\section{ablations}
video quality(if using gt data, using streampetr)
vae
encoding 

\section{visualtion}
occ inifinte city
long video 
controllable video generation
closed loop cases
